# Supplementary material for: Training Dynamic Exponential Family Models with Causal and Lateral Dependencies for Generalized Neuromorphic Computing
Source: arXiv:1810.08940 source file (2019-12-18)
Supplement: Supplementary file 1 [file appendix.tex]

\section*{Appendix}

\smallskip
\noindent {\bf Conditional and marginal distributions.}
For each unit $i$, its conditional probability (or firing probability) is given by 
\begin{align} \label{eq:DEF-unit-cond}
p(x_{i,t} | \bmx_{-i,t}, \bmx^{t-1}) &= p(x_{i,t} | \bmx_{\set{L}_i,t}, \bmalpha_{\set{P}_i,t-1}) \cr
&\propto \exp \Big\{ \big( \bmtheta_i + \sum_{j \in \set{P}_i} \sum_{k=1}^K \bfV_{j,i,k}^\top \bmalpha_{j,k,t-1} \big)^\top \bms_{i,t} + \sum_{j \in \set{L}_i} \bms_{j,t}^\top \bfU_{j,i} \bms_{i,t}  \Big\} := \exp \big\{ \bmr_{i,t}^\top \bms_{i,t} \big\},
\end{align}
where we use a notation $\bmx_{\set{A},t} = [x_{i,t}]_{i \in \set{A}}$ to denote a sub-vector of $\bmx_t$ for an arbitrary subset $\set{A} \subseteq \set{V}$; $\bmr_{i,t}$ to denote a conditioned energy of $i$ at time $t$ (similar to membrane potential in spiking neural networks) given by 
\begin{align} \label{eq:DEF-cond-energy}
\bmr_{i,t} := \bmtheta_i + \sum_{j \in \set{L}_i} \bfU_{j,i}^\top \bms_{j,t} + \sum_{j \in \set{P}_i} \sum_{k=1}^K \bfV_{j,i,k}^\top \bmalpha_{j,k,t-1}.
\end{align}
This conditioned energy at time $t$ depends on (i) the current signal $\bms_{j,t}$ of laterally connected units $j \in \set{L}_i$, (ii) the filtered inputs $\bmalpha_{j,t-1}$ from causally connected units $j \in \mathtt{Pa}_i$, and (iii) filtered output $\bmalpha_{i,t-1}$ of itself. Moreover, the associated local parameter for this conditioned energy of unit $i$ is $\Theta_i = \{ \bmtheta_i, \bfU_{\set{L}_i,i}, \bfV_{\set{P}_i,i} \}$.

Before to obtain the marginal distributions of nodes and edges at time $t$, we need following notations. Under the lateral graph $\set{G}_{\set{L}}$, we denote the set of units that are connected\footnote{From unit $i$, we can reach unit $m \in \set{C}_i$ through lateral connections and vice versa.} to unit $i$ by $\set{C}_i$, \ie, there exists a path between units $i$ and $m \in \set{C}_i$ where a path is a sequence of edges in $\set{E}_{\set{L}}$. We also denote by $\set{D}_i$ a set of units that are disconnected to unit $i$, thus it is obvious $\set{V} = \{i\} \cup \set{C}_i \cup \set{D}_i$ for every $i$. Then, units in $\{i\} \cup \set{C}_i$ and $\set{D}_i$ are {\em independent} given $\bmx^{t-1}$, \ie, 
\begin{align} \label{eq:DEF-indep-node}
p(\bmx_t | \bmx^{t-1}) &= p(x_{i,t}, \bmx_{\set{C}_i,t}, \bmx_{\set{D}_i,t} | \bmx^{t-1}) \cr &= p(x_{i,t}, \bmx_{\set{C}_i,t} | \bmx^{t-1}) p(\bmx_{\set{D}_i,t} | \bmx^{t-1}) \cr 
&= p(x_{i,t}, \bmx_{\set{C}_i,t} | \bmalpha_{\set{P}_{\{i\} \cup \set{C}_i}, t-1}) p(\bmx_{\set{D}_i,t} | \bmalpha_{\set{P}_{\set{D}_i}, t-1}).
\end{align}
Similarly, for each edge $(j,i) \in \set{E}_{\set{L}}$, units in $\{i,j\} \cup \set{C}_i \cup \set{C}_j$ and $\set{D}_i \cap \set{D}_j$ are independent given $\bmx^{t-1}$, \ie, 
\begin{align} \label{eq:DEF-indep-edge}
p(\bmx_t | \bmx^{t-1}) &= p(x_{i,t}, x_{j,t} , \bmx_{\set{C}_i \cup \set{C}_j, t} | \bmx^{t-1}) p(\bmx_{\set{D}_i \cap \set{D}_j, t} | \bmx^{t-1}) \cr 
&= p(x_{i,t}, x_{j,t} , \bmx_{\set{C}_i \cup \set{C}_j, t} | \bmalpha_{\set{P}_{\{i,j\} \cup \set{C}_i \cup \set{C}_j}, t-1}) p(\bmx_{\set{D}_i \cap \set{D}_j, t} | \bmalpha_{\set{P}_{\set{D}_i \cap \set{D}_j}, t-1}).
\end{align}

Now, we obtain marginal distributions for each unit $i \in \set{V}$ and each lateral connection $(j,i) \in \set{E}_{\set{L}}$ in following way. First for unit $i$, its marginal distribution $p_i(x_{i,t} | \bmx^{t-1})$ is computed using only the information of $\bmalpha_{\set{P}_{\{i\} \cup \set{C}_i}, t-1}$ from the given $\bmx^{t-1}$, \ie, 
\begin{align} \label{eq:DEF-marg-node}
p_i(x_{i,t} | \bmx^{t-1}) &= \sum_{\bmx_{-i,t}} p(\bmx_t | \bmx^{t-1}) \cr 
&= \sum_{\bmx_{\set{C}_i,t}} p(x_{i,t}, \bmx_{\set{C}_i,t} | \bmalpha_{\set{P}_{\{i\} \cup \set{C}_i}, t-1}) \sum_{\bmx_{\set{D}_i,t}} p(\bmx_{\set{D}_i,t} | \bmalpha_{\set{P}_{\set{D}_i}, t-1}) \cr 
&= \sum_{\bmx_{\set{C}_i,t}} p(x_{i,t}, \bmx_{\set{C}_i,t} | \bmalpha_{\set{P}_{\{i\} \cup \set{C}_i}, t-1}).
\end{align}
For $(j,i) \in \set{E}_{\set{L}}$, computing its marginal distribution $p_{j,i}(x_{j,t}, x_{i,t} | \bmx^{t-1})$ is done using only the information of $\bmalpha_{\set{P}_{\{i,j\} \cup \set{C}_i \cup \set{C}_j}, t-1}$ from given $\bmx^{t-1}$ as follows:
\begin{align} \label{eq:DEF-marg-edge}
p_{j,i}(x_{j,t},x_{i,t} | \bmx^{t-1}) &= \sum_{\bmx_{\set{V} \setminus \{i,j\},t}} p(\bmx_t | \bmx^{t-1}) 
= \sum_{\bmx_{\set{C}_i \cup \set{C}_j,t}} p(x_{i,t}, x_{j,t} , \bmx_{\set{C}_i \cup \set{C}_j, t} | \bmalpha_{\set{P}_{\{i,j\} \cup \set{C}_i \cup \set{C}_j}, t-1}).
\end{align}

\smallskip
\noindent {\bf Gibbs sampler for \eqref{eq:DEF}.}
The Gibbs sampler for $p(\bmx_t | \bmx^{t-1}, \Theta)$ generates a sequence of $M$ draws. Denote that $m$-th sample by $\bmx^{(m)}_t$. We proceed the sampling as follows. First, we begin with some initial value $\bmx^{(0)}_t$. At iteration $m$, the value $x^{(m)}_{i,t}$ of unit $i$ is drawn from the following conditional distribution given as
\begin{align}
x^{(m)}_{i,t} \sim p(x_{i,t} | x^{(m)}_{1,t},\cdots,x^{(m)}_{i-1,t}, x^{(m-1)}_{i+1,t},\cdots,x^{(m-1)}_{N_x,t}, \bmx^{t-1},\Theta ),
\end{align}
where the conditional distribution $p(x_{i,t} | \bmx_{\set{V} \setminus \{i\},t}, \bmx^{t-1}, \Theta)$ is computed as 
\begin{align} \label{eq:DEF-cond}
p(x_{i,t} | \bmx_{\set{V} \setminus \{i\},t}, \bmx^{t-1}, \Theta) 
%&= p(x_{i,t} | \bmx_{\set{L}_i,t} \bmalpha_{\set{P}_i},\Theta) \cr 
&\propto \exp \Big\{ \big( \bmtheta_j + \sum_{m \in \set{P}_j} \sum_{k=1}^K \bfV_{m,j,k}^\top \bmalpha_{m,k} \big)^\top \bms_{j,t} + \sum_{m \in \set{L}_j} \bms_{m,t}^\top \bfU_{m,j} \bms_{j,t} \Big\}.
\end{align}
This process is repeated until obtaining $M$ samples. The conditional distribution \eqref{eq:DEF-cond} is expressed by the conditioned energy $\bmr_{i,t}$ of unit $i$ at time $t$, \ie, 
\begin{align*}
p(x_{i,t} | \bmx_{\set{V} \setminus \{i\},t}, \bmx^{t-1}, \Theta) = p(x_{i,t} | \bmx_{\set{L}_i,t} \bmalpha_{\set{P}_i},\Theta) \propto \exp \big\{ \bmr_{i,t}^\top \bms_{i,t} \big\},
\end{align*}
where 
\begin{align*}
\bmr_{i,t} = \bmtheta_i + \sum_{j \in \set{P}_i} \sum_{k=1}^K \bfV_{j,i,k}^\top \bmalpha_{j,k} + \sum_{j \in \set{L}_i} \bfU_{j,i}^\top \bms_{j,t},
\end{align*}
which can be computed using local information $\bmx_{\set{L}_i,t}$ and $\bmalpha_{\set{P}_i}$. As a result, from the $M$ sample of the Gibbs sampler, the negative component of the gradients \eqref{eq:DEF-ll-grad} is approximated by
\begin{align}
\mathbb{E}_{\bfx_t \sim p(\bmx_t | \bmx^{t-1},\Theta)}[\bfs_{i,t} | \bmx^{t-1}] &= \frac{1}{M} \sum_{m=1}^M \bms_i(x^{(m)}_{i,t}), \cr  \mathbb{E}_{\bfx_t \sim p(\bmx_t | \bmx^{t-1},\Theta)}[\bfs_{j,t} \bfs_{i,t}^\top | \bmx^{t-1}] &= \frac{1}{M} \sum_{m=1}^M \bms_j(x^{(m)}_{j,t}) \bms_i(x^{(m)}_{i,t})^\top.
\end{align}

The Gibbs sampler from $p(x_{i,t},\bmx_{\mathtt{cn}_i,t} | \bmalpha_{\set{P}_{\set{C}_i},t-1},\Theta)$ in \eqref{eq:DEF-marginal-node} generates a sequence of $M$ draws, where we denote by $\bmx_{\set{C}_i,t}^{(m)}$ the $m$-th sample. We begin with some initial value $\bmx_{\set{C}_i,t}^{(0)}$ and at iteration $m$, the value $x_{j,t}^{(m)}$ of unit $j \in \set{C}_i$ is drawn based on the conditional distribution $p(x_{j,t} | \bmx_{\set{C}_i \setminus \{j\}}, \bmalpha_{\set{P}_{\set{C}_i},t-1},\Theta)$, see Appendix for details. We just here note that the conditional distribution of each unit $i$ required in the Gibbs sampler is 
\begin{align} \label{eq:DEF-cond-node}
p(x_{i,t} | \bmx_{\set{L}_i,t}, \bmalpha_{\set{P}_i,t-1},\Theta) 
& \propto \exp \Big\{ \big( \bmtheta_i + \sum_{j \in \set{P}_i} \sum_{k=1}^K \bfV_{j,i,k}^\top \bmalpha_{j,k,t-1} \big)^\top \bms_{i,t} + \sum_{j \in \set{L}_i} \bms_{j,t}^\top \bfU_{j,i} \bms_{i,t} \Big\} \cr  
& := \exp \big\{ \bmr_{i,t}^\top \bms_{i,t} \big\},
\end{align}
where we denote $\bmr_{i,t}$ the conditioned energy of unit $i$ at time $t$ by 
\begin{align} \label{eq:DEF-cond-energy}
\bmr_{i,t} = \bmtheta_i + \sum_{j \in \set{P}_i} \sum_{k=1}^K \bfV_{j,i,k}^\top \bmalpha_{j,k,t-1} + \sum_{j \in \set{L}_i} \bfU_{j,i}^\top \bms_{j,t}.
\end{align}
This process is repeated until obtaining $M$ samples, then the expectation over the node $i$'s marginals in \eqref{eq:DEF-ll-grad-th}, \eqref{eq:DEF-ll-grad-V} is computed by taking $M$ samples of neuron $i$:
\begin{align*}
\mathbb{E}_{\bfx_t \sim p(\bmx_t|\bmx^{t-1},\Theta)}[\bfs_{i,t}|\bmx^{t-1}] = \frac{1}{M} \sum_{m=1}^M \bms_{i}(x_{i,t}^{(m)}).
\end{align*}

Similarly, the Gibbs sampler from $p(x_{j,t},x_{i,t}, \bmx_{\mathtt{cn}_j \cup \mathtt{cn}_i,t} | \bmalpha_{\set{P}_{\set{C}_i \cup \set{C}_j},t-1}, \Theta)$ generates a sequence of $M$ draws $\{ \bmx_{\set{C}_j \cup \set{C}_i, t}^{(m)} \}_{m=1,\cdots,M}$ based on the conditional distribution \eqref{eq:DEF-cond-node}, then the negative component in \eqref{eq:DEF-ll-grad-U} is computed by taking $M$ samples of neurons $j$ and $i$:
\begin{align*}
\mathbb{E}_{\bfx_t \sim p(\bmx_t|\bmx^{t-1},\Theta)}[\bfs_{j,t} \bfs_{i,t}^\top |\bmx^{t-1}] = \frac{1}{M} \sum_{m=1}^M \bms_{j}(x_{j,t}^{(m)}) \bms_{i}(x_{i,t}^{(m)})^\top.
\end{align*}

%%% Local Variables: 
%%% mode: latex
%%% TeX-master: "main"
%%% End: 
