# Supplementary material for: Training Dynamic Exponential Family Models with Causal and Lateral Dependencies for Generalized Neuromorphic Computing
Source: arXiv:1810.08940 source file (2019-12-18)
Supplement: Supplementary file 2 [file snn_appendix.tex]

\subsection{Spiking Neural Networks} 
\label{sec:snn-model}

As an instance of the dynamic exponential family, we describe here a probabilistic model for Spiking Neural Networks (SNN), which include Generalized Linear Models (GLM) \cite{bagheri17:snn_first}, a version of Winner-Take-All (WTA) circuits \cite{kappel15:synaptic, habenschuss13:stdp}, and Boltzmann Machines for time-series \cite{osogami17:BMtime} as special cases. In an SNN, the signal $\rmx_{i,t}$ is binary, with value $1$ corresponding to a spike emitted by neuron $i$ at time $t$; and the sufficient statistic is given as $s_i(x_i) = x_i$. Note that accordingly, the filtered trace in \eqref{eq:filter-signal} is given by the scalar function as
\begin{align} \label{eq:SNN-filter-signal}
\alpha_{j,k,t} = \sum_{\delta=0}^{\tau-1} a_k^{[\delta+1]} x_{j,t-\delta},
\end{align}
which can be computed by means of only additions - an important computational advantage. 

The parameters $\bfV = \{\{v_{j,i,k}\}_{k=1,\ldots,K}\}_{(j,i) \in \set{E}_{\set{P}}}$ related to the directed graph in \eqref{eq:DEF-basis} are also scalar. The function $\sum_{k=1}^K v_{i,i,k} a_k^{[\delta]}$, for $\delta \in \{1,\ldots,\tau\}$, corresponds to the {\em feedback kernel} of neuron $i$, while the function $\sum_{k=1}^K v_{j,i,k} a_k^{[\delta]}$, for $\delta \in \{1,\ldots,\tau\}$, corresponds to the {\em synaptic kernel} applied on the synapse between neurons $j \in \set{P}_i$ and $i$. As seen in Fig.~\ref{fig:DEF_SNN}, the former acts as a feedback filter on the neuron's output, while the latter operates on the input spike trains.

The parameters $\bfU = \{u_{j,i}\}_{(j,i) \in \set{E}_{\set{L}}}$ describing the lateral connections are scalar quantities as well. A positive $u_{j,i}$ encourages simultaneous spiking of neurons $j$ and $i$; while a negative $u_{j,i}$ hinders the emission of simultaneous spikes by the two neurons. The GLM model \cite{bagheri17:snn_first} and Boltzmann machine for time-series \cite{osogami17:BMtime} typically assume no instantaneous correlations, \ie, they set $u_{j,i} = 0$ for all $(j,i) \in \set{E}_{\set{L}}$. In contrast, allowing for non-zero parameters $u_{j,i}$ makes it possible to implement more general models that account for forms of population coding \cite{spiridon01:lateral,habenschuss13:stdp}. For instance, a version of WTA circuits \cite{kappel15:synaptic,habenschuss13:stdp} considers competition among a subset of neurons through {\em lateral inhibition}, \ie, it sets $u_{j,i} = -\infty$ for all pair of neurons in the subset. As a result, when a neuron in the subset fires, it inhibits spiking from other neurons in the subset. 

\begin{comment}
\noindent {\bf Boltzmann machine for time-series.}
Our dynamic exponential family model \eqref{eq:DEF} cover a Boltzmann machine (BM) for time-series consisting of spiking neurons, \ie, DyBM introduced in \cite{osogami17:BMtime} according to the following coincidence: {\em (i)} DyBM model has no consideration of instantaneous correlations among neurons, \ie, all-zero matrices $\bfU$, {\em (ii)} no consideration of parameterization based on basis functions, {\em (iii)} \note{undirected causal connections??}, and {\em (iv)} the synapse weights $\bfW$ are assumed to have following form, which results a connection to a spiking-timing dependent plasticity (STDP) rule. 
\end{comment}

As conventional choices of basis functions, to parameterize the kernels, one can consider the raised cosine basis functions in Fig.~\ref{fig:ex_cos}. Alternatively, in order to connect the learning rule with the standard biologically-plausible Spiking-Timing Dependent Plasticity (STDP) rule with long term potentiation (LTP) and long term depression (LTD), we can consider $K=2M$ and the basis functions depicted in Fig.~\ref{fig:ex_stdp}, which are defined as \cite{osogami17:BMtime}
\begin{subequations} \label{eq:basis-stdp}
\begin{align}
a_{2k-1}^{[\delta]} &= \lambda_{2k-1}^{\delta-d} \cdot 1_{\{\delta \geq d\}}, \label{eq:basis-stdp-ltp} \\
a_{2k}^{[\delta]} &= -\lambda_{2k}^{-\delta} \cdot 1_{\{\delta < d\}}, \label{eq:basis-stdp-ltd}
\end{align}
\end{subequations}
% \begin{align}
% a_k^{[\delta]} = \lambda_k^{\delta -d} \cdot 1_{\{\delta \geq d\}}, &\quad ~\text{for}~ k=1,\cdots,M, \cr 
% a_k^{[\delta]} = -\mu_k^{-\delta} \cdot 1_{\{\delta < d\}}, &\quad ~\text{for}~ k=M+1,\cdots,2M.
% \end{align}
for $k=1,\ldots,M$, where $\delta \in \{1,\ldots,\tau\}$, and we have defined the decay rates $\lambda_{2k-1}, \lambda_{2k} \in (0,1]$ and the synaptic conduction delay $d \ll \tau$ of the signals between two arbitrary neurons. As we will detail in Section~\ref{sec:snn-learning} when discussing learning of the synaptic weights $\bfV = \{\{v_{j,i,2k-1}, v_{j,i,2k}\}_{k=1,\ldots,M}\}_{(j,i) \in \set{E}_{\set{P}}}$, the odd-numbered basis functions $a_{2k-1}^{[\delta]}$ for $k=1,\ldots,M$, describe LTP with decay rates $\lambda_{2k-1}$, while the even-numbered basis functions $a_{2k}^{[\delta]}$ for $k=1,\ldots,M$, describe LTD with decay rates $\lambda_{2k}$. As a practical note, when $\tau \rightarrow \infty$, the filtered signal \eqref{eq:SNN-filter-signal} with LTP-type basis functions, \ie, $\alpha_{j,2k-1,t}$ for $k=1,\ldots,M$, can be updated in recursive form as
\begin{align} \label{eq:ltp-trace}
\alpha_{j,2k-1,t} = \lambda_{2k-1} \cdot \big( \alpha_{j,2k-1,t-1} + x_{j,t-d} \big).
\end{align}

\begin{figure}[t]
  \centering
   \includegraphics[width=0.88\columnwidth]{fig/DEF_SNN_model}
  \caption{Internal structure of a unit or neuron. The illustration focuses on the case of binary units, which can model the behavior of a spiking neuron in an SNN.}
  \label{fig:DEF_SNN}
\end{figure}

\begin{comment}
\smallskip 
\noindent {\bf Example: Categorical unit.} \note{change to binary unit.}

Consider a categorical variable as a unit $i$ whose sample space is the set of $C_i$ individually identified items, simply represented as $\rmx_i \in \{1,\cdots,C_i\}$. As an exponential family, the categorical distribution of $\rmx_i$ is given by $p(x_i) \propto \exp \{ \bmtheta_i^\top \bms_i(x_i) \}$. The categorical unit $i$ has $C_i$ dimensional canonical parameter $\theta_i$ and sufficient statistics $\bms_i$ as follows:
\begin{align}
\bmtheta_i = [\log p_1, \cdots, \log p_{C_i}]^\top, \quad \bms_i(x_i) = [1_{\{x_i = 1\}}, \cdots, 1_{\{x_i = C_i\}}]^\top,
\end{align}
where $\sum_{c=1}^{C_i} p_c = 1$ and $1_{E}$ is the indicator function for the event $E$, \ie, $1_{\{x_i = c\}}$ evaluates to 1 if $x_i = c$ and $0$ otherwise. In particular, the sufficient statistics of the categorical unit having $x_i = c$ is a $C_i$ dimensional one-hot vector with a single $1$ value for $c$-th element and all the other elements $0$. Then, the categorical distribution is given by
\begin{align*}
p(x_i) = \exp \Big\{ \sum_{c=1}^{C_i} (\log p_c) \cdot 1_{\{x_i = c\}} \Big\} = \prod_{c=1}^{C_i} p_c^{1_{\{x_i = c\}}}.
\end{align*}
We can observe that $p(x_i = c) = p_c$, which means that $p_c$ is the probability that unit $i$ takes value of $c$ out of $C_i$ number of possible values.
\end{comment}

\subsection{Training of Spiking Neural Networks} \label{sec:snn-learning}

Here, we adapt the gradient-based rule described above for a general dynamic exponential family model to the SNN model introduced in Section~\ref{sec:snn-model}. We specifically focus on SNNs with no instantaneous correlations. Accordingly, the gradients of the log-likelihood \eqref{eq:DEF-ll-grad} can be written as 
\begin{align} \label{eq:snn-ll-grad}
\grad_{\theta_i} \ln p(\bmx_t | \bmalpha_{t-1},\Theta) = x_{i,t} - \sigma(r_{i,t}), \quad \grad_{v_{j,i,k}} \ln p(\bmx_t | \bmalpha_{t-1},\Theta) = \alpha_{j,k,t-1} \big( x_{i,t} - \sigma(r_{i,t}) \big),
\end{align}
where $r_{i,t} = \theta_i + \sum_{j \in \set{P}_i} \sum_{k=1}^K v_{j,i,k} \alpha_{j,k,t-1}$ is the so-called {\em membrane potential} of neuron $i$ at time $t$, and $\sigma(\cdot)$ is the sigmoid function, \ie, $\sigma(x) = 1/( 1+\exp(-x))$. 

A gradient-based learning scheme based on \eqref{eq:snn-ll-grad} has a direct relationship with the standard STDP rule when one chooses the STDP basis functions in \eqref{eq:basis-stdp}. Accordingly, the gradient of the log-likelihood for the weights $v_{j,i,k}$ is given as 
\begin{subequations} \label{eq:snn-ll-grad-stdp}
\begin{align}
\grad_{v_{j,i,2k-1}} \ln p(\bmx_t | \bmalpha_{t-1},\Theta) &= \sum_{\delta=d}^{\tau} \lambda_{2k-1}^{\delta-d} x_{j,t-\delta} \cdot \Big( x_{i,t} - \sigma(r_{i,t}) \Big) \label{eq:snn-ll-grad-stdp-ltp} \\
\grad_{v_{j,i,2k}} \ln p(\bmx_t | \bmalpha_{t-1},\Theta) &= \sum_{\delta=1}^{d-1} \lambda_{2k}^{-\delta} x_{j,t-\delta} \cdot \Big( -x_{i,t} + \sigma(r_{i,t}) \Big), \label{eq:snn-ll-grad-stdp-ltd}
\end{align}
\end{subequations}
for $k=1,\cdots,M$. This learning rule relates to the standard STDP rule in that the amount of the change in the weight between two causally connected neurons depends on the precise timings when the two neurons fired. In particular, the odd-numbered synaptic weights $v_{j,i,2k-1}$, which are associated with the basis functions \eqref{eq:basis-stdp-ltp} describing LTP, are increased when a spike $x_{i,t}=1$ of neuron $i$ occurs after a small time $\delta$ from a spike $x_{j,t-\delta}$ of neuron $j \in \set{P}_i$ as long as $\delta$ is larger than the synaptic delay $d$. In contrast, the even-numbered synaptic weights $v_{j,i,2k}$ associated with the basis functions \eqref{eq:basis-stdp-ltd} describing LTD decreases when neuron $j \in \set{P}_i$ spikes $\delta < d$ time instants before a spike from neuron $i$, with the decrease being larger as $\delta$ approaches the synaptic delay $d$. In \eqref{eq:snn-ll-grad-stdp}, the amount of change of synaptic weights also depends on the neuron $i$'s average activity $\sigma(r_{i,t})$, which can be interpreted as a form of {\em homeostatic plasticity} \cite{watt10:homeostatic} in that it regulates an average neuronal firing rate around some desirable set-point value. In \eqref{eq:snn-ll-grad-stdp-ltp}, the increase of LTP weight is small if the neuron $i$ is already likely to fire, \ie, $\sigma(r_{i,t})$ is large, while in \eqref{eq:snn-ll-grad-stdp-ltd} the decrease of LTD weight is small if the neuron $i$'s average activity is low. 

%\note{check the details... and the interpretation of $\sigma$-terms compared to the standard STDP... Homeostatic plasticity?}

%In contrast, associated with the basis functions \eqref{eq:basis-stdp-ltd} describing LTD, the even-numbered synaptic weights $v_{j,i,2k}$ for $k=1,\cdots,M$, are increased, \ie, LTD gets stronger, when the non-spike $x_{i,t}=0$ of neuron $i$ is given. Then, the neuron $i$ becomes less likely to fire when the filtered signal from $j$ is expected to reach soon, \ie, the first term in \eqref{eq:snn-ll-grad-stdp-ltd} is large. 

%{\bf NOTE:} Training of two-layer SNNs in supervised learning problems?
